# Supplementary material for: An Assessment of Approximate Methods for Anharmonic Free Energies
Source: arXiv:1906.06524 ancillary file (2019-06-15)
Supplement: Supplementary file 1 [file si.pdf]

# An Assessment of Approximate Methods for Anharmonic Free Energies

Venkat Kapil,[*,†] Edgar Engel,[*,†] Mariana Rossi,[‡] and Michele Ceriotti[†]

†*Laboratory of Computational Science and Modeling, Institut des Matériaux, École Polytechnique Fédérale de Lausanne, 1015 Lausanne, Switzerland*

‡*Fritz Haber Institute of the Max Planck Society, Faradayweg 4-6, 14195 Berlin, Germany*

**S1 Diamond and Lonsdaleite** **S-3**
S1.1 Computational Details . . . . . S-3
S1.1.1 Independent mode approximation (IMF) . . . . . S-3
S1.1.2 Vibrational self-consistent field (VSCF) . . . . . S-3
S1.1.3 Self-consistent phonons (SCP) . . . . . S-4
S1.1.4 Thermodynamic integration (QTI) . . . . . S-4
S1.2 Convergence with respect to system size . . . . . S-4
S1.3 Computational cost of SCP . . . . . S-5

**S2 Ice XIh and Ice XIc** **S-5**
S2.1 Computational Details . . . . . S-5
S2.1.1 Independent mode approximation (IMF) . . . . . S-6
S2.1.2 Vibrational self-consistent field (VSCF) . . . . . S-6
S2.1.3 Self-consistent phonons (SCP) . . . . . S-6
S2.1.4 Thermodynamic integration (QTI) . . . . . S-6
S2.2 Convergence with respect to system size . . . . . S-7
S2.3 Blue-shift of Librations . . . . . S-7

**S3 Paracetamol forms I and II** **S-8**
S3.1 Computational Details . . . . . S-8
S3.1.1 Independent mode approximation (IMF) . . . . . S-8
S3.1.2 Vibrational self-consistent field (VSCF) . . . . . S-8
S3.1.3 Self-consistent phonons (SCP) . . . . . S-8
S3.1.4 Thermodynamic integration (QTI) . . . . . S-9

**S4 Analysis of efficiency of thermodynamic integration** **S-9**

**S5 Relative stability of proton ordered phases of ice** **S-11**

**S6 Influence of noise in the potential energy landscapes on IMF** **S-12**

**References** **S-13**

# S1 Diamond and Lonsdaleite

## S1.1 Computational Details

Lattices containing $N = 2$ (4), $8, 16, 32, 64$ atoms for diamond (lonsdaleite) were constructed using the `make_super_cell` function implemented in ASE[1] and further optimized (with fixed cell) using a L-BFGS algorithm[2] implemented in i-PI.[3] Tolerances of $10^{-10}$ Hartree and $10^{-6}$ Hartree/Bohr for the potential energy and the force components were respectively used for the minimization algorithm. The Hessians of the harmonic references were calculated using a finite difference scheme implemented in i-PI.[3] Displacements of 0.005 Bohr along each Cartesian coordinate ensured converged normal mode frequencies. The acoustic sum rule was imposed to project out the three translational modes. The harmonic reference was used as a starting point for all free energy methods.

### S1.1.1 Independent mode approximation (IMF)

The potential energy was mapped out by displacing the system along each normal mode until the sampled energy exceeded $n_E = 16$ times their respective harmonic thermal vibrational energy, which corresponds to about four times the harmonic RMS displacements. The potential was interpolated on a regular grid of 501 points using cubic splines. The convergence with respect to the number of simple harmonic oscillator (SHO) states and the sampling density $f$ was performed automatically within the code.

### S1.1.2 Vibrational self-consistent field (VSCF)

The 2D potential energy surfaces along pairs of normal modes were mapped using $n_E = 16$ and $f = 0.5$, which led to converged results for IMF. The interpolation was performed on a regular grid of $101 \times 101$ points as the pair-wise coupling corrections $V^{(2)}(q_i, q_j) - V^{(1)}(q_i) - V^{(2)}(q_j)$ were found to be more slowly varying than independent mode corrections. A basis of 15 SHO states – that gave converged results for IMF – was used to solve the mean-field Schrodinger's equation.

### S1.1.3 Self-consistent phonons (SCP)

For supercells containing $N = 2$ (4), 8, 16, 32, 64 atoms $N_s = 100$ (100), 100, 100, 200, 500 Monte Carlo samples per SCP iteration were used for diamond (lonsdaleite). Within each iteration multiple optimization steps for the average forces and the Hessian were performed until the former were converged up to their statistical errors or until the batch weights became smaller than 0.9.

### S1.1.4 Thermodynamic integration (QTI)

The reversible work to "switch-on" the anharmonic part of the potential was calculated from six classical MD simulations with the Kirkwood parameters $\lambda = 0.0, 0.2, 0.4, 0.6, 0.8, 1.0$. A white noise Langevin thermostat with time constant $\tau = 100$ was used to enforce canonical sampling. A BAOAB[4] scheme as described in Ref.[5] was used to integrate the equations of motion with a time step of 1 fs. The mean force was calculated from the harmonic and anharmonic components of the potential at every step.

The work done to "switch-on" quantum effects was calculated from 10 PIMD simulations with the mass scaling factor $g = 0.01, 0.04, 0.09, \ldots, 0.81, 1.00$ such that $\sqrt{g}$ uniformly samples $(0, 1]$ as suggested by Ceriotti and Markland.[6] To get well converged results, we performed Suzuki-Chin PIMD[7] simulations with 16 beads using a time step of 0.25 fs and a PILE-L thermostat with $\tau = 100$ fs. The mean force was calculated using the centroid virial kinetic energy every 1 fs.

## S1.2 Convergence with respect to system size

Fig. S1 shows the convergence of the anharmonic free energy of diamond and lonsdaleite and their free energy difference as a function of system size. For $N = 32$, the free energy difference between diamond and lonsdaleite is converged to around 1 meV / atom.

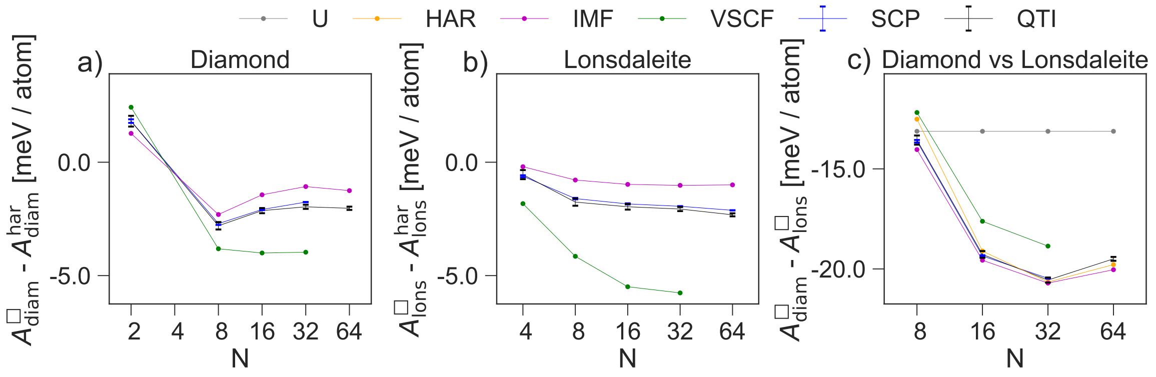


Figure S1: Panels (a) and (b) show the convergence of the anharmonic free energy of diamond and lonsdaleite, calculated at 300 K using IMF (pink), VSCF (green) and SCP (blue), as function of number of atoms $N$ in the supercell. Panel (c) similarly shows the convergence of the free energy difference between diamond and lonsdaleite calculated using the the aforementioned methods including HAR and the static lattice approximation (U). Numerically exact results calculated using a path integral thermodynamic integration scheme are shown in black.

### S1.3 Computational cost of SCP

Fig. S2 shows the dependence of the computational cost (as defined in section IV.B) of SCP on the number of atoms in the simulation cell when pseudo random numbers and Sobol sequences are used for importance sampling, respectively. Since the error rate for the latter behaves asymptotically as $O\left(\log(N_s)^d/N_s\right)$, for a large enough $d$ the scaling behaviour of the SCP scheme becomes exponential with respect to system size.

## S2 Ice XIh and Ice XIc

### S2.1 Computational Details

Lattices containing $N = 2\,(4), 8, 16, 32, 64$ for XIc (XIh) were constructed using the `make_super_cell` function implemented in ASE[1] and further geometry optimized (with fixed cell) using a L-BFGS algorithm.[2] The same tolerances for geometry optimizations and finite displacements as in subsection S1.1 were found to lead to converged harmonic references.

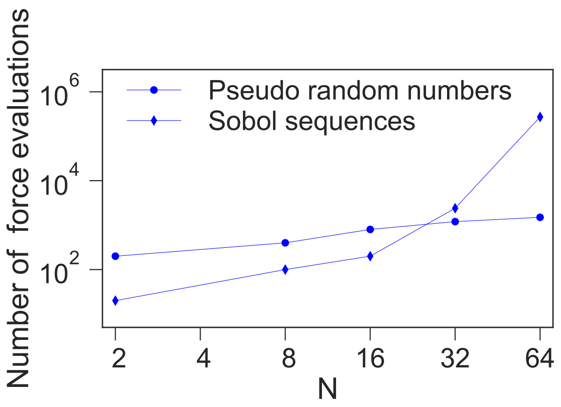


Figure S2: Computational costs in the case of diamond in terms of the number of energy and force evaluations for SCP, using pseudo random numbers (round) and Sobol sequences (diamond) for Monte Carlo sampling, with number of atoms (N) in the simulation cell. Solid lines are guides for the eye. In all cases the free energy was converged to within 10% of the reference TI results for 64 atoms with respect to all relevant convergence parameters.

#### S2.1.1 Independent mode approximation (IMF)

Same as subsection S1.1.1

#### S2.1.2 Vibrational self-consistent field (VSCF)

Same as subsection S1.1.2

#### S2.1.3 Self-consistent phonons (SCP)

$N_s$ = 1000 samples per SCP iteration were used for all the simulation cells of XIc and XIh with all other parameters matching those in subsection S1.1.3.

#### S2.1.4 Thermodynamic integration (QTI)

The reversible work to "switch-on" the anharmonic part of the potential was calculated from six classical molecular dynamics (MD) simulations with the Kirkwood parameters $\lambda = 0.0, 0.2, 0.4, 0.6, 0.8, 1.0$. A white noise Langevin thermostat with $\tau$ = 100 was used to enforce canonical sampling. A BAOAB[4] scheme was used to integrate the equations of motion with a time step of 0.5 fs. The mean force was calculated every step.

The work done to "switch-on" quantum effects was calculated from 10 path integral MD (PIMD) simulations with the mass scaling factor $g = 0.01, 0.04, 0.09, \ldots, 0.81, 1.00$, i.e. $\sqrt{g}$ uniformly selected in $(0, 1]$. To get well converged results, we performed Suzuki-Chin PIMD[7] simulations with 96 beads using a time step of 0.25 fs and a PILE-L thermostat with $\tau = 100$ fs. The mean force was calculated every 1 fs.

## S2.2 Convergence with respect to system size

As shown in Fig. S3, for $N = 8$, the free energy difference between XIh and XIc is converged to around 1 meV / molecule for all the methods.

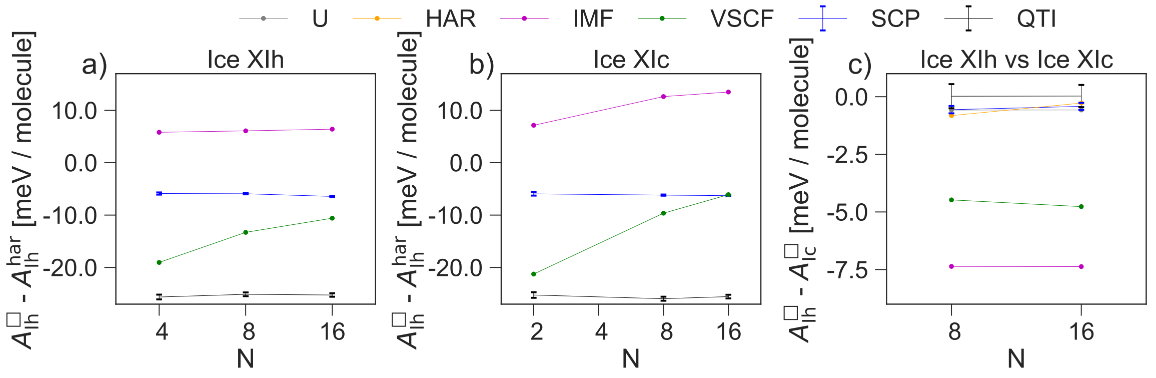


Figure S3: Panels (a) and (b) show the convergence of the anharmonic free energy of XIh and XIc forms of ice at 70 K using IMF (pink), VSCF (green) and SCP (blue), as function of number of water molecules $N$ in the supercell. Panel (c) similarly shows the convergence of the free energy difference between XIh and XIc calculated using the the aforementioned methods including HAR and the static lattice approximation (U). Numerically exact results calculated using a path integral thermodynamic integration scheme are shown in black.

## S2.3 Blue-shift of Librations

The stiffening of the librational motion is evidenced directly by the positive anharmonic correction along the modes as shown in Fig. S4. In the case of SCP the blue shift – as indicated by the increase in the free energy – is observed for the trial Hamiltonian which highlights that the amplitude of the librational motion is underestimated, potentially leading to errors in the total free energy.

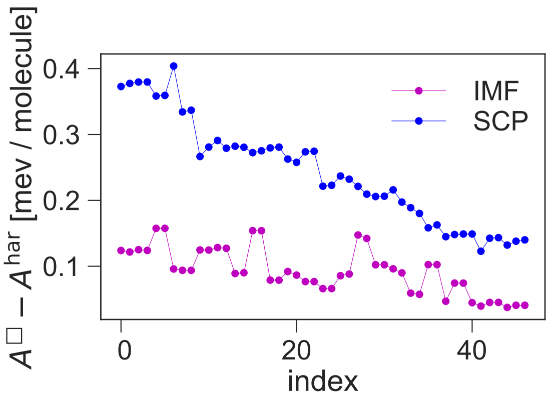


Figure S4: The anharmonic free energy associated with the librational modes of ice XIh at 70 K calculated using IMF (pink) and the SCP trial Hamiltonian (blue) for a supercell containing 16 molecules of water.

# S3 Paracetamol forms I and II

## S3.1 Computational Details

Lattices containing $N = 4$ and $N = 8$ molecules of paracetamol for forms I and II were used following the system size convergence performed in Ref.[3] The lattice constants were rescaled to their respective experimental values and the positions of atoms were optimized. The remaining workflow is same as the one described subsection S1.1.

### S3.1.1 Independent mode approximation (IMF)

Same as subsection S1.1.1

### S3.1.2 Vibrational self-consistent field (VSCF)

Same as subsection S1.1.2

### S3.1.3 Self-consistent phonons (SCP)

$N_s = 5000$ samples per SCP iteration were used for both forms of paracetamol with all other parameters matching those in subsection S1.1.3.

#### S3.1.4 Thermodynamic integration (QTI)

The reversible work to "switch-on" the anharmonic part of the potential was calculated from six classical molecular dynamics (MD) simulations with the Kirkwood coupling coefficient $\lambda = 0.0, 0.2, 0.4, 0.6, 0.8, 1.0$ at 10 K and was found to be almost zero. A correction of $-k_B T \log 3$ was added to account for the degeneracy of the three conformers. The free energy at 300K was calculated by performing a thermodynamic integration[8] over 27 intermediate temperatures (chosen as a geometric progression) with parallel tempering[9] to ensure ergodic sampling of the three conformers. All simulations were performed with a white noise Langevin thermostat with $\tau = 100$. A BAOAB[4] scheme was used to integrate the equations of motion with a time step of 0.5 fs. The mean force was calculated every 20 fs. The workflow was tested to reproduce the classical anharmonic free energies of the lattices used in Ref.[3]

The work done to "switch-on" quantum effects was calculated from 10 path integral MD (PIMD) simulations with the mass scaling factor $g = 0.01, 0.04, 0.09, \ldots, 0.81, 1.00$. To get well converged results, we used Suzuki-Chin PIMD[7] with 16 beads using a time step of 0.25 fs and a PILE-L thermostat with $\tau = 100$ fs, and a BAOAB integrator. The kinetic energy was printed out every 1 fs. The mean force was calculated every 1 fs.

# S4 Analysis of efficiency of thermodynamic integration

The total quantum anharmonic free energy obtained as a sum of the centre of mass, classical harmonic, classical anharmonic and quantum anharmonic contributions to the free energies is:

$$A = A^{\mathrm{cm}} + A^{\mathrm{har}}_{\mathrm{cl}} + \Delta A_{\mathrm{cl}} + \Delta A_{\mathrm{qn}} \tag{S4.1}$$

$$= A^{\mathrm{cm}} + A^{\mathrm{har}}_{\mathrm{cl}} + \int_0^1 \mathrm{d}\lambda \, \left\langle V - V^{\mathrm{har}} \right\rangle_{H^\lambda} + \int_0^1 \mathrm{d}g \; g^{-1} \left\langle \hat{T} - T_{\mathrm{cl}} \right\rangle_{\hat{H}^g}. \tag{S4.2}$$

We first consider the error in the classical anharmonic free energy. Let us say that the thermodynamic integration is performed using $n_\lambda$ values of $\lambda$. The mean force for each of these values is assumed

to be estimated from $N_s^{\text{cl}}$ samples obtained from MD simulations printed at a stride of $S^{\text{cl}}$. The total number of force evaluations required to calculate $\Delta A_{\text{cl}}$ is

$$C^{\text{cl}} = n_\lambda N_s^{\text{cl}} S^{\text{cl}}. \tag{S4.3}$$

The associated error is $\sqrt{\frac{\sigma_{\text{cl}}^2}{N_s^{\text{cl}}}}$ where $\sigma_{\text{cl}}^2$ is total uncertainty obtained by appropriately propagating the variance and the auto-correlation time of $\left\langle V - V^{\text{har}} \right\rangle_{H^\lambda}$ into the quadrature formula used for approximating the integral. Similarly, the number of force evaluations required to compute the quantum anharmonic free energy is

$$C^{\text{qn}} = n_g N_s^{\text{qn}} S^{\text{qn}} P \tag{S4.4}$$

where $P$ represents the number of beads used in the PIMD simulations. The error associated with $\Delta A_{\text{qn}}$ is $\sqrt{\frac{\sigma_{\text{qn}}^2}{N_s^{\text{qn}}}}$ where $\sigma_{\text{qn}}^2$ is also estimated appropriately. The total error in $A$ is therefore:

$$\sigma = \sqrt{\frac{\sigma_{\text{cl}}^2}{N_s^{\text{cl}}} + \frac{\sigma_{\text{qn}}^2}{N_s^{\text{qn}}}} \tag{S4.5}$$

and the total number of force evaluations are:

$$C = n_\lambda N_s^{\text{cl}} S^{\text{cl}} + n_g N_s^{\text{qn}} S^{\text{qn}} P \tag{S4.6}$$

The minimum number of force evaluations for a fixed target accuracy $\sigma$ are obtained by simply optimizing $C$ w.r.t $N_s^{\text{cl}}$ or $N_s^{\text{cl}}$. In practice we first ran long simulations for each point of the thermodynamic integration to get reliable estimates of $\sigma_{\square}^2$ (knowing that they are biased by $N_s^{\square}$). We then solved for the optimal values of $N_s^{\square}$. The errors computed *a posteriori* were found to be comparable to $\sigma$.

## S5 Relative stability of proton ordered phases of ice

We calculate the Helmholtz free energy of three high density polymorphs of ice, II[10], IX[11] and XV[12] with respect to that of XIh at 70K. This allows us to study the accuracy of the approximate methods across systems that are structurally more dissimilar than the ones considered in the manuscript. We use unit cells containing 12, 12 and 10 molecules of water for ice II, IX and XV, respectively at their experimental densities. As shown in Fig. S5, all approximate methods perform worse than the harmonic approximation. While IMF and VSCF give quantitatively incorrect relative free energies, SCP does not even give the qualitatively result.

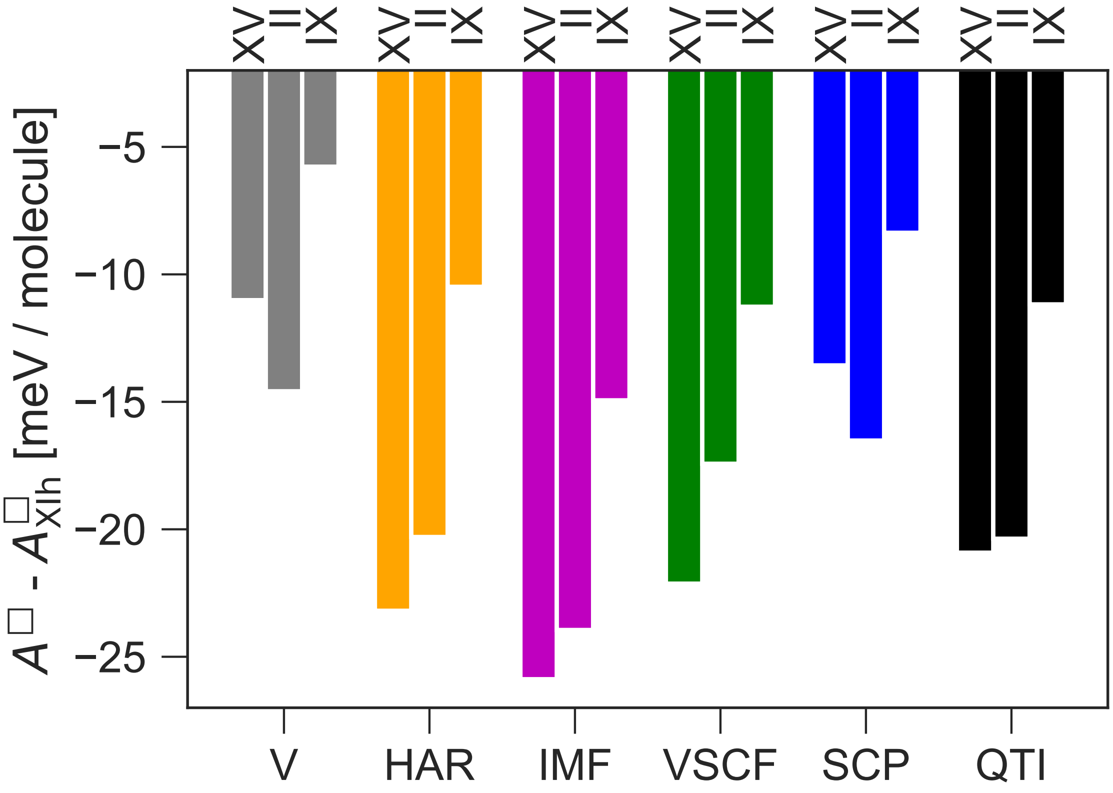


Figure S5: The difference between the Helmholtz free energy of ice II, IX and XV and ice XIh at 70 K using various approximate methods including the static lattice approximation (V) and the harmonic approximation (HAR). Numerically exact results calculated using a path integral thermodynamic integration scheme (QTI) are shown in black.

## S6 Influence of noise in the potential energy landscapes on IMF

PPPM accuracy parameters of $1.0^{-6}$ and $1.0^{-4}$ for the maximum fractional error in the force components are considered for calculating the potential energy of form II of paracetamol. The normal modes are obtained using the higher accuracy parameter by estimating the Hessian using finite differences. As shown in Fig. S6, the system is displaced along the lowest frequency normal mode and the potential energy curve is calculated using both PPPM parameters. The use of the lower accuracy parameter leads to noise in the potential energy landscape that is of the order of 0.5 meV. This results in a discrepancy of 1.07 mev in the IMF free energy.

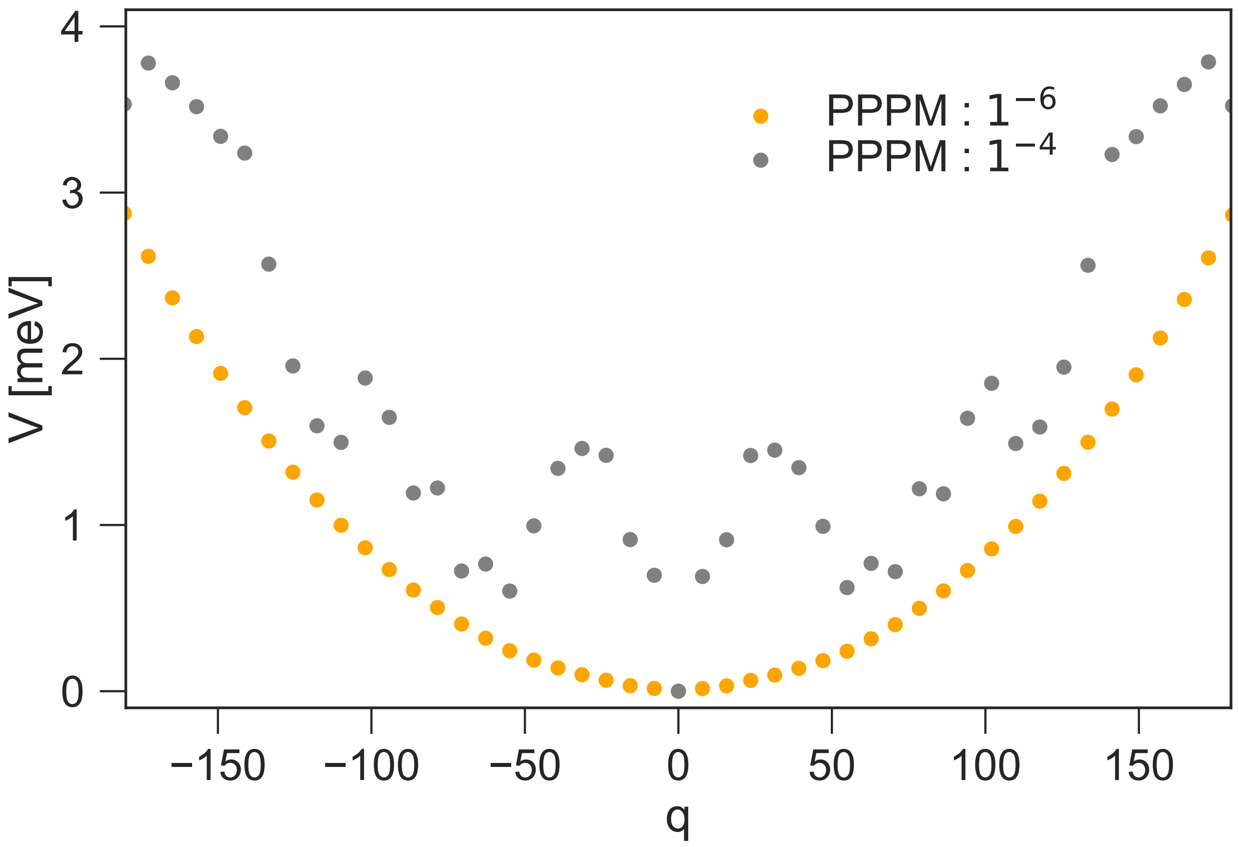


Figure S6: The potential energy curve obtained by displacing the lowest frequency normal mode of paracetamol form II (in units of the harmonic root mean square displacement) using PPPM accuracy parameters of $1.0^{-4}$ and $1.0^{-6}$ fractional error in the force components.

# References


(1) Larsen, A. H. et al. The atomic simulation environment—a Python library for working with atoms. *Journal of Physics: Condensed Matter* **2017**, *29*, 273002.

(2) Liu, D. C.; Nocedal, J. On the limited memory BFGS method for large scale optimization. *Mathematical Programming* **1989**, *45*, 503–528.

(3) Rossi, M.; Gasparotto, P.; Ceriotti, M. Anharmonic and Quantum Fluctuations in Molecular Crystals: A First-Principles Study of the Stability of Paracetamol. *Physical Review Letters* **2016**, *117*, 115702.

(4) Leimkuhler, B.; Matthews, C. Robust and efficient configurational molecular sampling via Langevin dynamics. *The Journal of Chemical Physics* **2013**, *138*, 174102.

(5) Kapil, V.; Wieme, J.; Vandenbrande, S.; Lamaire, A.; Speybroeck, V. V.; Ceriotti, M. Modeling the structural and thermal properties of loaded metal-organic frameworks. An interplay of quantum and anharmonic fluctuations. *arXiv* **2019**,

(6) Ceriotti, M.; Markland, T. E. Efficient methods and practical guidelines for simulating isotope effects. *The Journal of Chemical Physics* **2013**, *138*, 014112.

(7) Kapil, V.; Behler, J.; Ceriotti, M. High order path integrals made easy. *Journal of Chemical Physics* **2016**, *145*, 234103.

(8) Moustafa, S. G.; Schultz, A. J.; Kofke, D. A. Very fast averaging of thermal properties of crystals by molecular simulation. *Physical Review E* **2015**, *92*.

(9) Sugita, Y.; Okamoto, Y. Replica-exchange molecular dynamics method for protein folding. *Chemical Physics Letters* **1999**, *314*, 141–151.

(10) Kamb, B. Ice. II. A proton-ordered form of ice. *Acta Crystallographica* **1964**, *17*, 1437–1449.

(11) Kamb, B.; Prakash, A. Structure of ice III. *Acta Crystallographica Section B Structural Crystallography and Crystal Chemistry* **1968**, *24*, 1317–1327.

(12) Kamb, B. Structure of Ice VI. *Science* **1965**, *150*, 205–209.
